# Supplementary material for: Fairness-Aware Reinforcement Learning (FAReL): A Framework for Transparent and Balanced Sequential Decision-Making
Source: arXiv:2509.22232 source file (2025-09-26)
Supplement: Supplementary file 1 [file appendix_fraud_extra.tex]

\subsection{Fraud Detection (Extra)}
\label{appendix:fraud_results_extra}

\begin{landscape}
% [inline block 0: 8 envs, 77292 chars -> data_tex | \begin{longtable}{lllrrrrrrrr} \caption{The statistical summary of the representative subset of fraud detection policies...]

\end{scriptsize}
