# Supplementary material for: Fairness-Aware Reinforcement Learning (FAReL): A Framework for Transparent and Balanced Sequential Decision-Making
Source: arXiv:2509.22232 source file (2025-09-26)
Supplement: Supplementary file 2 [file appendix_job_extra.tex]

\subsection{Job hiring (Extra)}
\label{appendix:job_results_extra}

\begin{landscape}
% [inline block 0: 11 envs, 99362 chars -> data_tex | \begin{longtable}{lllrrrrrrrr} \caption{The statistical summary of the representative subset of job hiring policies, for...]

\end{scriptsize}
